# Supplementary material for: Critical Filling Factor for the Formation of a Quantum Wigner Crystal Screened by a Nearby Layer
Source: arXiv:1808.06246 ancillary file (2018-08-21)
Supplement: Supplementary file 1 [file FFF_SM_20180710_arXiv.pdf]

# Supplemental Material to "Critical Filling Factor for the Formation of a Quantum Wigner Crystal Screened by a Nearby Layer"

H. Deng, L.N. Pfeiffer, K.W. West, K.W. Baldwin, and M. Shayegan
*Department of Electrical Engineering, Princeton University*

(Dated: August 1, 2018)

In this Supplemental Material, we present the details of the Landau level alignment (LLA) model which describes the oscillations of the layer densities in the bilayer electron system (BLES) as we sweep the magnetic field ($B$) [1]. With the asymmetric doping, the BLES has a very asymmetric charge distribution in the two layers, leading to a majority layer with the density $n_{Maj}$ and a minority layer with the density $n_{Min}$ [Fig. S1(a)]. $n_{Maj}$ and $n_{Min}$ can be tuned using the top and bottom gates. At $B = 0$, the Fermi levels ($E_F$) in two layers are aligned at thermal equilibrium. Because $n_{Maj}$ and $n_{Min}$ are unequal, there is an energy difference $\Delta E$ between the conduction-band bottoms of the two layers [Fig. S1(b)]. Once $B$ is applied, the energy level in each layer quantizes into a set of LLs. Because $n_{Maj}$ and $n_{Min}$ are different, the filling factors of the majority and minority layers ($\nu_{Maj}$ and $\nu_{Min}$) are also different. However, thermal equilibrium keeps $E_F$ in the two layers aligned, resulting in a $\Delta E$ that becomes dependent on $B$, as Figs. S1(c-d) illustrate. As a function of $B$, $\Delta E$ oscillates, leading to an interlayer charge transfer from the minority layer to the majority layer [Fig. S1(c)] or vice versa [Fig. S1(d)]. At sufficiently high $B$, $E_F$ in both layers reaches the lowest LLs, i.e. both layers are in the extreme quantum limit (EQL). In the EQL, $\Delta E$ equals zero and no longer changes [Fig. S1(e)], ending the charge transfer.

In a simple, classical capacitance model, at a given $B$, the amount of transferred charge $Q(B) = (C/e) \times [\Delta E(0) - \Delta E(B)]$, where $C = \epsilon/\widetilde{d}$ is the interlayer capacitance, $\epsilon$ is the dielectric constant of GaAs/AlGaAs, $\widetilde{d}$ is the center-to-center distance between two layers, and $\Delta E(B)$ is $\Delta E$ at the given $B$. $Q(B) > 0$ means that the charge transfers from the minority to the majority layer, and vice versa for $Q(B) < 0$. In the calculation for a given $B$, we test all the possible combinations of $n_{Maj}$ and $n_{Min}$ under the constraint that the total density $n_{tot} = n_{Maj} + n_{Min}$ is fixed and independent of $B$, until we find the correct values of $n_{Maj}$ and $n_{Min}$ that satisfy $n_{Maj} - n_{Maj,0} = -(n_{Min} - n_{Min,0}) = Q(B)/e$, where $n_{Maj,0}$ and $n_{Min,0}$ are $n_{Maj}$ and $n_{Min}$ at $B = 0$. In practice, we use a self-consistent calculation to find the correct values of $n_{Maj}$ and $n_{Min}$. Starting with an arbitrary combination of $n_{Maj}$ and $n_{Min}$ (e.g., $n_{Maj,0}$ and $n_{Min,0}$), $\nu_{Maj}$ and $\nu_{Min}$ at the given $B$ is calculated directly. Based on $\nu_{Maj}$ and $\nu_{Min}$, we determine $E_F$ in each layer as the energy of the highest occupied energy level. The difference between $E_F$ of the two layers gives $\Delta E(B)$. Using the value of $\Delta E(B)$ and the capacitance model described above, $Q(B)$ is calculated. We then update $n_{Maj}$ and $n_{Min}$ with the new values $[n_{Maj} + Q(B)/e$ and $n_{Min} - Q(B)/e]$, and repeat the calculation. When the values of $n_{Maj}$ and $n_{Min}$ become stable (to within 0.1%), the final $n_{Maj}$ and $n_{Min}$ are the results of the calculation for this given $B$.

More rigorously, the evolution of LLs and the interlayer change transfer is determined by the subband densities rather than the layer densities [2, 3]. However, in *all* of our samples, the subband densities are essentially the layer densities because of the strong asymmetry and negligible tunneling between the two layers [4]. The LLA model described above is therefore reasonably accurate. Indeed, in the low-field regime where $\nu_{Maj} > 2$, the layer densities predicted by the LLA model match the experimental data fairly well. We would like to emphasize that, the LLA model only requires three input parameters: $\widetilde{d}$ which is determined by the wafer structure, and the zero-field layer densities ($n_{Maj,0}$ and $n_{Min,0}$) which are experimentally measured via the Shubnikov-de Haas oscillations. There are no fitting parameters in the LLA model calculations.

According to the LLA model, the minority layer should be depleted completely at intermediate $B$ by the interlayer charge transfer, when $n_{Min,0}$ is low enough (i.e., $\leq Q(B)$). Indeed, this is the case for *all* the data discussed in this study: we sufficiently decreased $n_{Min,0}$ via gate-voltage biases so that the interlayer charge transfer predicted by the LLA model should deplete the minority layer for $\nu_{Maj} \leq 2$ [black horizontal lines above $\simeq 3$ T in Figs. 1(a) and 2(a-c)]. However, a clear deviation between the calculation results and the experimental data emerges when $\nu_{Maj} \leq 2$ [red horizontal lines in Figs. 1(a) and 2(a-c)]. This deviation indicates that the electrons are retained in the minority layer at high $B$ *starting from* $\nu_{Maj} = 2$ by a mechanism which is not included in the LLA model. Based on the observation of the commensurability oscillations at high fields [Fig. 1(d)] and the incompressibility of a pinned Wigner crystal, we deduce that this mechanism is the formation of the Wigner crystal in the minority layer.

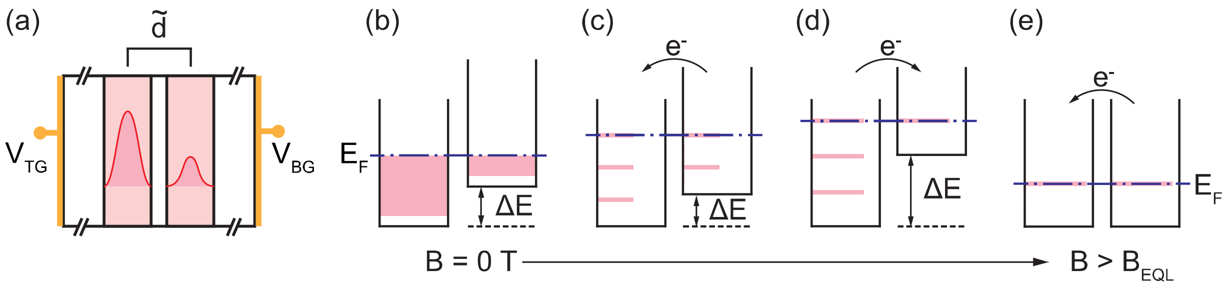


FIG. S1. (a) Schematic of the structure for sample A. The right and left pink-shaded regions indicate the GaAs quantum wells while the white regions indicate the AlGaAs barrier. The red curves show the charge distribution. $V_{TG}$ and $V_{BG}$ are the voltage biases applied on the top and bottom gates respectively. $\widetilde{d}$ is the center-to-center distance between quantum wells. (b)-(e) Landau level alignment and interlayer charge transfer induced by magnetic field $B$. $E_F$ is the Fermi level of the BLES. $\Delta E$ is the energy difference between the two layers. $B_{EQL}$ is the field when both layers reach the EQL. The arrow between the quantum wells indicates the direction of interlayer charge transfer compared to the case at $B = 0$ [Fig. S1(b)] (after Ref. [1]).

[1] H. Deng, Y. Liu, I. Jo, L. N. Pfeiffer, K. W. West, K. W. Baldwin, and M. Shayegan, Phys. Rev. B **96**, 081102 (2017).
[2] A. G. Davies, C. H. W. Barnes, K. R. Zolleis, J. T. Nicholls, M. Y. Simmons, and D. A. Ritchie, Phys. Rev. B **54**, R17331 (1996).
[3] Y. Liu, J. Shabani, D. Kamburov, M. Shayegan, L. N. Pfeiffer, K. W. West, and K. W. Baldwin, Phys. Rev. Lett. **107**, 266802 (2011).
[4] X. Ying, S. R. Parihar, H. C. Manoharan, and M. Shayegan, Phys. Rev. B **52**, R11611 (1995).
